# Supplementary material for: Disordered collective motion in dense assemblies of persistent particles
Source: arXiv:2201.04902 ancillary file (2022-06-23)
Supplement: Supplementary file 1 [file sm.pdf]

# Supplementary Material for "Disordered collective motion in dense assemblies of persistent particles"

Yann-Edwin Keta,[1] Robert L. Jack,[2,3] and Ludovic Berthier[1,2]

[1]*Laboratoire Charles Coulomb (L2C), Université de Montpellier, CNRS, 34095 Montpellier, France*
[2]*Yusuf Hamied Department of Chemistry, University of Cambridge, Lensfield Road, Cambridge CB2 1EW, United Kingdom*
[3]*Department of Applied Mathematics and Theoretical Physics, University of Cambridge, Wilberforce Road, Cambridge CB3 0WA, United Kingdom*

(Dated: June 23, 2022)

## CAGE-RELATIVE DISPLACEMENTS

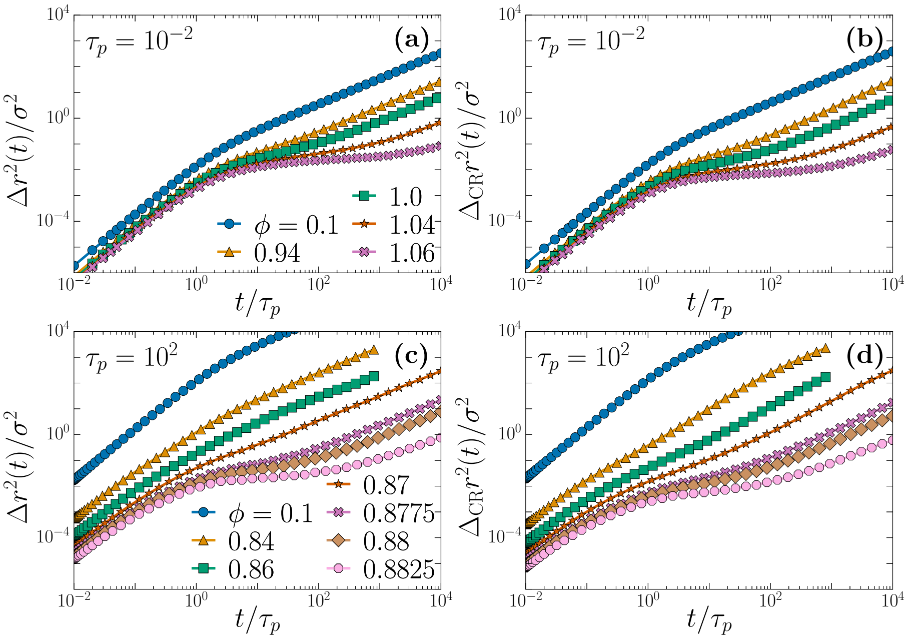


FIG. S1. (a, c) Mean squared displacements for different packing fractions $\phi$, at persistence time (a) $\tau_p = 10^{-2}$ and (b) $\tau_p = 10^2$ – these are Fig. 2(a,b) of main text. (b, d) Cage-relative mean squared displacements for different packing fractions $\phi$, at persistence time (b) $\tau_p = 10^{-2}$ and (d) $\tau_p = 10^2$.

As shown by Shiba *et al.* [1], particle displacements in dense passive 2D systems can be strongly affected by long wavelength sound modes. This effect is especially pronounced in very large systems, which support very long-wavelength modes. One way to control for this effect is to measure the cage-relative MSD [2]

$$\Delta_{\mathrm{CR}} r^2(t) = \frac{1}{N} \sum_i \left\langle \left| \boldsymbol{r}_i(t) - \boldsymbol{r}_i(0) - \frac{1}{N_i} \sum_j (\boldsymbol{r}_j(t) - \boldsymbol{r}_j(0)) \right|^2 \right\rangle, \tag{1}$$

where the second sum is taken over the $N_i$ nearest neighbours $j$ of particle $i$, determined by Voronoi tesselation. $\Delta_{\mathrm{CR}} r^2(t)$ differs significantly from the absolute MSD $\Delta r^2(t)$ in cases where the long-wavelength modes are dominant.

Fig. S1 shows cage-relative MSDs. These are similar to absolute MSDs, so we infer that the particle displacements are not controlled primarily by long wavelength modes. This confirms that (absolute) displacements are appropriate observables for characterising structural relaxation of the liquid. (We would expect long-wavelength modes to have a bigger effect in simulations of larger systems: in that case we would suggest to control for the presence of long-wavelength modes by working throughout with cage-relative displacements, or other suitable observables [3]).

## TEMPORAL VELOCITY CORRELATIONS

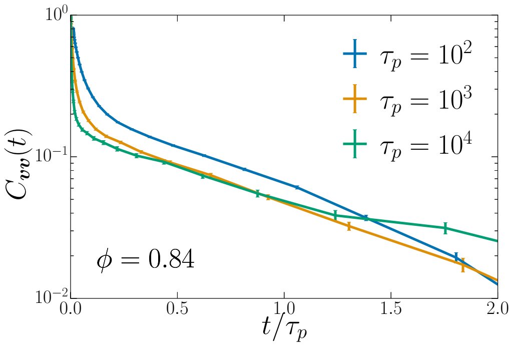


FIG. S2. Temporal velocity correlations at $\phi = 0.84$ for different persistence times $\tau_p$.

Velocity correlations depend on several factors, which can depend nontrivially on both the packing fraction $\phi$ and the persistence time $\tau_p$ (*e.g.* elastic moduli). Qualitative observations in our setting show that $\tau_p$ is the typical time scale of these correlations, consistently with theories of velocity correlations in active glasses [4] and active liquids [5].

## SUPPLEMENTARY MOVIES

- **SuppMovie1.mov**: Fraction of a system of $N = 4096$ particles, at $\tau_p = 10^3$ and $\phi = 0.84$. Each frame are separated by a time $\delta t = 0.05\tau_p$ and the frame rate is 5fps.
- **SuppMovie2.mov**: Same system of $N = 4096$ particles, at $\tau_p = 10^3$ and $\phi = 0.84$. Particles are given a color (black or white) according to their position at $t = 0$ following a checkerboard pattern for better visualisation of the motion. Each frame are separated by a time $\delta t = 0.05\tau_p$ and the frame rate is 5fps.


[1] Hayato Shiba, Yasunori Yamada, Takeshi Kawasaki, and Kang Kim, "Unveiling Dimensionality Dependence of Glassy Dynamics: 2D Infinite Fluctuation Eclipses Inherent Structural Relaxation," Physical Review Letters **117**, 245701 (2016).

[2] Bernd Illing, Sebastian Fritschi, Herbert Kaiser, Christian L. Klix, Georg Maret, and Peter Keim, "Mermin–Wagner fluctuations in 2D amorphous solids," Proceedings of the National Academy of Sciences **114**, 1856–1861 (2017).

[3] Hayato Shiba, Takeshi Kawasaki, and Akira Onuki, "Relationship between bond-breakage correlations and four-point correlations in heterogeneous glassy dynamics: Configuration changes and vibration modes," Physical Review E **86**, 041504 (2012).

[4] Silke Henkes, Kaja Kostanjevec, J Martin Collinson, Rastko Sknepnek, and Eric Bertin, "Dense active matter model of motion patterns in confluent cell monolayers," Nature Communications **11**, 1–9 (2020).

[5] Umberto Marini Bettolo Marconi, Andrea Puglisi, and Lorenzo Caprini, "Hydrodynamics of simple active liquids: The emergence of velocity correlations," arXiv preprint arXiv:2105.13832 (2021).
